# Supplementary material for: A Kernel-Based Approach for Accurate Steady-State Detection in Performance Time Series
Source: arXiv:2506.04204 source file (2025-06-04)
Supplement: Supplementary file 1 [file appendix.tex]

\section{Detection of the Step Index}\label{sec:appStepDet}

\begin{figure}[!ht]
\caption{The process of kernel-based step-down detection. The choice of step is described in-depth by \Cref{alg:stepChoice}.}
\label{fig:stepDetection}
% Resize the entire diagram to fit within the column width
\resizebox{\columnwidth}{!}{
\begin{tikzpicture}[node distance=1.8cm, line width=1mm, font=\small] % Reduced node distance

% Define block styles
\tikzstyle{startstop} = [rectangle, rounded corners, minimum width=3cm, minimum height=1cm, text centered, draw=black, fill=myred!60]
\tikzstyle{process} = [rectangle, minimum width=3cm, minimum height=0.8cm, text centered, draw=black, fill=mygreen!60] % Reduced height
\tikzstyle{decision} = [ellipse, minimum width=4cm, minimum height=1.5cm, text centered, draw=black, fill=myyellow!60] % Changed to ellipse
\tikzstyle{arrow} = [thick,->,>=stealth]

% Nodes
\node (start) [startstop] {Start};
\node (lk) [right of=start, font=\small, xshift=3cm]  {LK: Large Kernel};  % Abbreviation
\node (sk) [below of=lk, font=\small, yshift=1cm] {SK: Small Kernel};
\node (slk) [below of=sk, font=\small, yshift=1cm]  {SLK: Step from LK};  % Abbreviation
\node (ssk) [below of=slk, font=\small, yshift=1cm] {SSK: Step from SK};

\node (subtractavg) [process, below of=start] {Subtract mean of data};
\node (largekernel) [process, below of=subtractavg] {Convolve with LK};
\node (smallkernel) [process, below of=largekernel] {Convolve with SK};
\node (checklarge) [decision, below of=smallkernel, yshift=-0.5cm] {SLK equal to max idx?}; % Smaller yshift
\node (largelast) [process, right of=checklarge, xshift=3cm] {Set SLK to -1}; % Reduced xshift
\node (checksmall) [decision, below of=checklarge, yshift=-1cm] {SSK equal to max idx?}; % Smaller yshift
\node (smalllast) [process, right of=checksmall, xshift=3cm] {Set SSK to -1}; % Reduced xshift
\node (compare) [decision, below of=checksmall, yshift=-1cm] {SLK equal to SSK?}; % Smaller yshift
\node (discardlarge) [process, right of=compare, xshift=3cm] {Discard SLK}; % Reduced xshift
\node (processlarge) [decision, below of=compare, yshift=-1cm] {SLK larger than -1?}; % Smaller yshift
\node (largedetected) [process, right of=processlarge, xshift=2.5cm] {Process SLK}; % Reduced xshift
\node (smalldetected) [process, below of=largedetected] {Process SSK};
\node (choosestep) [process, below of=smalldetected] {Choose step based on comparison};
\node (end) [startstop, below of=choosestep] {Return step index};

% Arrows
\draw [arrow] (start) -- (subtractavg);
\draw [arrow] (subtractavg) -- (largekernel);
\draw [arrow] (largekernel) -- (smallkernel);
\draw [arrow] (smallkernel) -- (checklarge);
\draw [arrow] (checklarge) -- node[above] {Yes} (largelast);
\draw [arrow] (checklarge) -- node[below] {No} (checksmall);
\draw [arrow] (checksmall) -- node[above] {Yes} (smalllast);
\draw [arrow] (checksmall) -- node[below] {No} (compare);
\draw [arrow] (compare) -- node[above] {Yes} (discardlarge);
\draw [arrow] (compare) -- node[below] {No} (processlarge);
\draw [arrow] (processlarge) -- (largedetected);
\draw [arrow] (largedetected) -- (smalldetected);
\draw [arrow] (smalldetected) -- (choosestep);
\draw [arrow] (choosestep) -- (end);

\end{tikzpicture}
} % End of resizebox
\end{figure}

\begin{algorithm}[h]
\caption{Step Choice Algorithm}
\label{alg:stepChoice}

% Variables abbreviation
\textbf{Input:} 
\begin{itemize}
    \item $d$: Data (timeseries) array
    \item $w$: Window size (\texttt{step\_win\_size})
    \item $n$: Data length
    \item $l$: Large kernel step index
    \item $s$: Small kernel step index
\end{itemize}

\textbf{Output:} Step index $i$ (\texttt{step\_idx})

\begin{algorithmic}[1]
\If{$l > -1$}
    \If{$s > l$}
        \State $tmp \gets s$
        \State $s \gets l$
        \State $l \gets tmp$
    \ElsIf{$s = l$}
        \State \Return $s$
    \EndIf
    \If{$s = 0$}
        \State \Return $l$
    \EndIf

    \State $L_{\text{left}} \gets d[\max(l - w, 0) : l + 1]$
    \State $L_{\text{right}} \gets d[l + 1 : \min(l + w + 1, n)]$
    \State $L_{\text{diff}} \gets \text{median}(L_{\text{left}}) - \text{median}(L_{\text{right}})$

    \State $i \gets s$
    \State $R_{\text{med}} \gets \text{median}(d[l+1:])$

    \If{$\text{median}(d[s + 1 : l]) > 2.0 \times |L_{\text{diff}}| + R_{\text{med}}$}
        \State $i \gets l$
    \EndIf
\ElsIf{$s > -1$}
    \State $i \gets s$
\EndIf

\If{$\text{median}(d[:i]) - \text{median}(d[i:]) < |\text{median}(d)| / 2$}
    \If{$i > s$}
        \State $i \gets s$
    \Else
        \State \Return -1
    \EndIf
\EndIf

\State \Return $i$

\end{algorithmic}
\end{algorithm}

\section{\texorpdfstring{$S_2$}{S2} Sobol's Indices}\label{sec:appSobolS2}
\begin{table}[ht]
\caption{The second-order Sobol's indices $S_2$}
\label{tab:sobolS2}
\begin{tabular}{@{}r@{}|@{}c@{}|@{}c@{}c@{}c@{}}
\cline{2-5}
\multicolumn{1}{l|}{} &
  prob\_win\_size &
  \multicolumn{1}{c|}{step\_win\_size} &
  \multicolumn{1}{c|}{t\_crit} &
  \multicolumn{1}{c|}{prob\_threshold} \\ \hline
\multicolumn{1}{|r|}{outlier\_win\_size} &
  \begin{tabular}[c]{@{}c@{}}0 \\ (-0.06, 0.07)\end{tabular} &
  \multicolumn{1}{c|}{\begin{tabular}[c]{@{}c@{}}0 \\ (-0.01, 0.02)\end{tabular}} &
  \multicolumn{1}{c|}{\begin{tabular}[c]{@{}c@{}}0.02 \\ (-0.05, 0.08)\end{tabular}} &
  \multicolumn{1}{c|}{\begin{tabular}[c]{@{}c@{}}0.01 \\ (-0.05, 0.07)\end{tabular}} \\ \hline
\multicolumn{1}{|r|}{prob\_threshold} &
  \begin{tabular}[c]{@{}c@{}}0.04 \\ (-0.03, 0.11)\end{tabular} &
  \multicolumn{1}{c|}{\begin{tabular}[c]{@{}c@{}}0 \\ (-0.01, 0.01)\end{tabular}} &
  \multicolumn{1}{c|}{\begin{tabular}[c]{@{}c@{}}0.13 \\ (0.04, 0.23)\end{tabular}} &
   \\ \cline{1-4}
\multicolumn{1}{|r|}{t\_crit} &
  \begin{tabular}[c]{@{}c@{}}0.07 \\ (0, 0.14)\end{tabular} &
  \multicolumn{1}{c|}{\begin{tabular}[c]{@{}c@{}}0 \\ (-0.01, 0.01)\end{tabular}} &
   &
   \\ \cline{1-3}
\multicolumn{1}{|r|}{step\_win\_size} &
  \begin{tabular}[c]{@{}c@{}}-0.03 \\ (-0.09, 0.04)\end{tabular} &
   &
   &
   \\ \cline{1-2}
\end{tabular}
\end{table}
